# Supplementary material for: Regret-Optimal Control under Partial Observability
Source: arXiv:2311.06433 source file (2023-11-14)
Supplement: Supplementary file 1 [file AppendixC.tex]

\section{The Strictly-Causal Solution}\label{sec::SCsol}

\begin{lemma}\label{lemma:decomposition-SC}
The transfer matrix $A(z) = M^{1/2}(z)Q_2(z)W^{-/2}(z)$ can be expressed as a sum of two strictly-causal and an anticausal transfer matrices given by
 \begin{align}
    \overline{C}_1&= - M^{1/2}(z) G_2^\ast U_1F_S \c{F_S} F_SU_2 H^\ast R_W^{-\ast/2} \nn \\
    &= z^{-1} C_1(z)\nn\\
    \overline{C}_2&= -  R_M^{1/2} K_M \c{F_E} \overline{U}_3 G_A\nn \\
 \overline{A}(z)&=  z^{-1} \overline{H}_A \a{F_A^\ast}G_A
 \end{align}
where $U_1,U_2$ are given in \eqref{eq:Lyapunov} and $\overline{U}_3$ solves the equation $\overline{U}_3 = F_E\overline{U}_3 F_a^\ast + G_E \tilde{h}_A$ with $\tilde{h}_A = G_2^\ast \begin{pmatrix}
        U_1F_SU_2&I 
    \end{pmatrix}$ and constant $\overline{H}_A = - R_M^{1/2} (\tilde{h}_A -  K_M U_3F_A^\ast)$.
\end{lemma}

\begin{proof}[Proof of Lemma \ref{lemma:decomposition-SC}]
For the strictly causal scenario, we write  \eqref{eq:proof_decompo_6product} as 
%(the constants are temporarily omitted)
%  \begin{align}\label{eq:proof_red_sc_6prod}
%      & [F_S^\ast \a{F_S^\ast} U_1 + U_1F_S \c{F_S} + U_1]G_1G_1^\ast \a{F_W^\ast} \nn  \\
%      &=  [z^{-1}\a{F_S^\ast} U_1 + U_1F_S \c{F_S} ]G_1G_1^\ast \a{F_W^\ast} \nn \\
%     %  &=  z^{-1}\a{F_S^\ast} U_1G_1G_1^\ast \a{F_W^\ast} + U_1F_S \c{F_S} G_1G_1^\ast \a{F_W^\ast}\nn \\
%     %  &= z^{-1}\a{F_S^\ast} U_1G_1G_1^\ast \a{F_W^\ast} + U_1F_S [\c{F_S} F_SU_2 + U_2 F_W^\ast \a{F_W^\ast} + U_2]\nn \\
%      &= z^{-1}\a{F_S^\ast} U_1G_1G_1^\ast \a{F_W^\ast} + U_1F_S [\c{F_S} F_SU_2 + U_2 z^{-1} \a{F_W^\ast} ]\nn \\
%     %  &= z^{-1}\a{F_S^\ast} U_1G_1G_1^\ast \a{F_W^\ast} + U_1F_S U_2 z^{-1} \a{F_W^\ast} + U_1F_S \c{F_S} F_SU_2 \nn \\
%      &= z^{-1} \begin{pmatrix}
%         U_1F_SU_2&I 
%     \end{pmatrix}
%     \a{\begin{pmatrix}
%         F_W^\ast & 0\\
%         U_1G_1G_1^\ast & F_S^\ast
%     \end{pmatrix}}
%     \begin{pmatrix}
%     I \\
%     0 
%     \end{pmatrix} + U_1F_S \c{F_S} F_SU_2.
% \end{align}
% By adding the constants to \eqref{eq:proof_red_sc_6prod}, we can write \eqref{eq:proof_decompo_6product} as
\begin{align}
    & z^{-1} \tilde{h}_A \a{F_A^\ast}G_A \nn\\
    &\ + G_2^\ast U_1F_S \c{F_S} F_SU_2 H^\ast R_W^{-\ast/2},
 \end{align}
 with $\tilde{h}_A \triangleq G_2^\ast \begin{pmatrix}
        U_1F_SU_2&I 
    \end{pmatrix}$. The anticausal transfer matrix $z^{-1} \tilde{h}_A \a{F_A^\ast}G_A$ can be combined with $-M^{1/2}(z)$ as
 \begin{align}
    & - M^{1/2}(z) z^{-1} \tilde{h}_A \a{F_A^\ast}G_A\nn \\
    &= - z^{-1}R_M^{1/2} (I + K_M \c{F_E}G_E) \tilde{h}_A \a{F_A^\ast}G_A  \nn\\
    &= - z^{-1} R_M^{1/2} \tilde{h}_A \a{F_A^\ast}G_A \nn\\
    &\ - z^{-1}  R_M^{1/2} K_M \c{F_E}G_E \tilde{h}_A \a{F_A^\ast}G_A \nn \\
     &\stackrel{(a)}= - z^{-1} R_M^{1/2} \{\tilde{h}_A \a{F_A^\ast} \nn\\
     & + K_M [\c{F_E} F_E \overline{U}_3 + \overline{U}_3F_A^\ast\a{F_A^\ast} + \overline{U}_3]\}G_A \nn \\
    %  &= - R_M^{1/2} \tilde{h}_A \a{F_A^\ast}G_A z^{-1} 
    %  -  R_M^{1/2} K_M \overline{U}_3F_A^\ast\a{F_A^\ast} G_A z^{-1}\nn \\
    %  &-  R_M^{1/2} K_M (\c{F_E} F_E + I)\overline{U}_3 G_A z^{-1}\nn \\
    %  &= - z^{-1} R_M^{1/2} (\tilde{h}_A +  K_M \overline{U}_3 F_A^\ast) \a{F_A^\ast}G_A -  R_M^{1/2} K_M \c{F_E} \overline{U}_3 G_A \nn \\
     &\triangleq z^{-1} \overline{H}_A \a{F_A^\ast}G_A -  R_M^{1/2} K_M \c{F_E} \overline{U}_3 G_A,
 \end{align}
 where in $(a)$ $\overline{U}_3$ solves $\overline{U}_3 = F_E\overline{U}_3 F_a^\ast + G_E \tilde{h}_A$ and in the last step we denote $\overline{H}_A \triangleq - R_M^{1/2} (\tilde{h}_A +  K_M \overline{U}_3F_A^\ast)$.

To summarize the decomposition for the strictly causal scenario, the anticausal part is
\begin{align}
    \overline{A}(z)&=  z^{-1} \overline{H}_A \a{F_A^\ast}G_A,
\end{align}
and the strictly causal functions are given by
\begin{align}
    \overline{C}_1(z)&= - M^{1/2}(z) G_2^\ast U_1F_S \c{F_S} F_SU_2 H^\ast R_W^{-\ast/2}\nn \\
    \overline{C}_2(z)&= -  R_M^{1/2} K_M \c{F_E} \overline{U}_3 G_A.
\end{align}
\end{proof}
\begin{lemma}[Solution to the Nehari problem with $\overline{A}(z)$]\label{lemma:nehari_sc}
The solution to the Nehari problem with $\overline{A}(z) = z^{-1} \overline{H}_A\a{F_A^\ast}G_A$ is 
\begin{align}
    \overline{C}_N(z)&= \textcolor{red}{z^{-1} \overline{H}_A \Pi(\overline{F}_N \c{\overline{F}_N} + I) \overline{K}_N}\\
    &= \overline{H}_A \Pi \c{\overline{F}_N} \overline{K}_N
\end{align}
where
\begin{align}
    \overline{K}_N &= (I - F_A \overline{Z}_\gamma F_A^\ast\Pi)^{-1}F_A \overline{Z}_\gamma G_A\\
    \overline{F}_N &= F_A - \overline{K}_NG_A^\ast
\end{align}
and $\overline{Z}_\gamma$ and $\Pi$ are the solutions to the Lyapunov equation
\begin{align}
    \overline{Z}_\gamma&= F_A \overline{Z}_\gamma F_A^\ast + \gamma^{-2}\overline{H}_A^\ast \overline{H}_A\nn \\
    \Pi&= F_A^\ast \Pi F_A + G_AG_A^\ast.
\end{align}
\end{lemma}
Note that $\Pi$ is the same as the one for the causal scenario.
\begin{proof}[Proof of Lemma \ref{lemma:nehari_sc}]
Note that the Nehari problem can be reformulated as follows
\begin{align}
    \min_{\text{S.C.} \ C(z)} \| C(z)- \overline{A}(z)\|&=     \min_{\text{S.C.} \ C(z)} \| z C(z)- z \overline{A}(z)\|\nn\\
    &= \min_{\text{causal} \ C'(z)} \| C'(z)- z \overline{A}(z)\|.
\end{align}
Using this derivation, we can directly apply the solution to the Nehari problem from \textcolor{red}{Theorem \ref{}} and multiply the resulted solution with $z^{-1}$.
\end{proof}
\begin{theorem}\label{th:ss_sc}[Regret-Optimal Controller: Strictly-Causal]
The regret-optimal strictly causal (Youla) controller is given by
\begin{align}
    \xi_{i+1} &= A \xi_i + B \alpha_i \nn \\
    q_i&= C\xi_i 
\end{align}
with 
\begin{align}
    A&= \begin{pmatrix}
     F_W & 0 & 0 & 0\\
     - F_SU_2 H^\ast R_W^{-1}H &F_S&0&0\\
     -  \overline{K}_N R_W^{-/2}H  &0& \overline{F}_N & 0 \\
     - \overline{U}_3 G_AR_W^{-/2}H &0& G_E R_M^{-/2}\overline{H}_A \Pi & F_M
    \end{pmatrix},\nn \\ 
    B&= \begin{pmatrix}
     K_W\\ F_SU_2 H^\ast R_W^{-1} \\ \overline{K}_N R_W^{-/2} \\ \overline{U}_3 G_AR_W^{-/2}
    \end{pmatrix},\nn \\
    C&= \begin{pmatrix}
     0& - G_2^\ast U_1F_S & R_M^{-/2}\overline{H}_A \Pi & -K_M
    \end{pmatrix}
\end{align}
\end{theorem}
\begin{proof}[Proof of Theorem \ref{th:ss_sc}]
By Theorem \ref{th:reduction}, the regret-optimal controller for the strictly causal scenario is 
\begin{align}\label{eq:proof_th_sc_main}
    Q_{sc}(z)&= M^{-1/2}(z) (\overline{C}_N(z) + \overline{C}_1 + \overline{C}_2)W^{1/2}(z)
\end{align}
with the functions 
\begin{align}
    M^{-1/2}(z)&= (I - K_M \c{F_M}G_E)R_M^{-/2}\nn \\
    \overline{C}_N(z)&= \overline{H}_A \Pi \c{\overline{F}_N} \overline{K}_N \nn \\
    W^{1/2}(z) &= R_W^{-/2}(I - H \c{F_W}K_W) \nn \\
    \overline{C}_1&= - M^{1/2}(z) G_2^\ast U_1F_S \c{F_S} F_SU_2 H^\ast R_W^{-\ast/2}\nn \\
    \overline{C}_2&= -  R_M^{1/2} K_M \c{F_E} \overline{U}_3 G_A.
\end{align}
We start by simplifying the first two terms in \eqref{eq:proof_th_sc_main}
\begin{align}\label{eq:proof_sc_th_3prod}
    M^{-1/2}(z) \overline{C}_1 R_W^{-/2} &= - G_2^\ast U_1F_S \c{F_S} F_SU_2 H^\ast R_W^{-1} \nn \\
  M^{-1/2}(z) \overline{C}_2 R_W^{-/2} 
%  &= - (I + K_M \c{F_E}G_E)^{-1} K_M \c{F_E} \overline{U}_3 G_AR_W^{-/2}  \nn \\
 &= - K_M \c{F_M} \overline{U}_3 G_AR_W^{-/2}.
    %  &M^{-1/2}(z) \overline{K}_N(z) R_W^{-/2} \\
    %  &= (I - K_M \c{F_M}G_E)R_M^{-/2}\overline{H}_A \Pi \c{\overline{F}_N} \overline{K}_N R_W^{-/2}.\nn
\end{align}
The second term in \eqref{eq:proof_sc_th_3prod} can be combined with the Nehari term as
\begin{align}
    &M^{-1/2}(z) (\overline{C}_2 + \overline{C}_N) R_W^{-/2} = \begin{pmatrix}
     R_M^{-/2}\overline{H}_A \Pi & -K_M
    \end{pmatrix}\nn\\
    &\cdot \c{\begin{pmatrix}
     \overline{F}_N & 0 \\
     G_E R_M^{-/2}\overline{H}_A \Pi & F_M
    \end{pmatrix}}
    \begin{pmatrix}
     \overline{K}_N R_W^{-/2} \\ \overline{U}_3 G_AR_W^{-/2}
    \end{pmatrix},
\end{align}
and by also adding the first line of \eqref{eq:proof_sc_th_3prod}, we get 
\begin{align}\label{eq:proof_th_sc_prod_final}
    &M^{-1/2}(z) (\overline{C}_1 + \overline{C}_2 + \overline{C}_N) R_W^{-/2}\nn\\
    &=\begin{pmatrix}
      - G_2^\ast U_1F_S & R_M^{-/2}\overline{H}_A \Pi & -K_M
    \end{pmatrix} \\
    &\cdot \left(zI - \begin{pmatrix}
     F_S&0&0\\
     0& \overline{F}_N & 0 \\
     0& G_E R_M^{-/2}\overline{H}_A \Pi & F_M
    \end{pmatrix}\right)^{-1}
    \begin{pmatrix}
     F_SU_2 H^\ast R_W^{-1} \\ \overline{K}_N R_W^{-/2} \\ \overline{U}_3 G_AR_W^{-/2}
    \end{pmatrix}.\nn
    \end{align}
Finally, we need to multiply \eqref{eq:proof_th_sc_prod_final} with $R_W^{1/2}W^{1/2}(z)$. To this end, we use the general formula in \eqref{eq:proof_gen_formula1} to combine \eqref{eq:proof_th_sc_prod_final} with $R_W^{1/2}W^{1/2}(z)$ as appears in Theorem~\ref{th:ss_sc}.
% \begin{align}
%     &Q_{sc}(z)= \begin{pmatrix}
%      0& - G_2^\ast U_1F_S & R_M^{-/2}\overline{H}_A \Pi & -K_M
%     \end{pmatrix}\nn\\
%     &\cdot     \left(zI - \begin{pmatrix}
%      F_W & 0 & 0 & 0\\
%      - F_SU_2 H^\ast R_W^{-1}H &F_S&0&0\\
%      -  \overline{K}_N R_W^{-/2}H  &0& \overline{F}_N & 0 \\
%      - \overline{U}_3 G_AR_W^{-/2}H &0& G_E R_M^{-/2}\overline{H}_A \Pi & F_M
%     \end{pmatrix}\right)^{-1}\nn\\
%     &\cdot \begin{pmatrix}
%      K_W\\ F_SU_2 H^\ast R_W^{-1} \\ \overline{K}_N R_W^{-/2} \\ \overline{U}_3 G_AR_W^{-/2}
%     \end{pmatrix}.\nn
% \end{align}
\end{proof}
